# Supplementary material for: Thermo-remnant magnetization assisted switching response
Source: arXiv:1902.06911 source file (2019-02-19)
Supplement: Supplementary file 1 [file Supplementary_materials_3.pdf]

# 1 Experimental Methodology

$SmCrO_3$ polycrystallites are synthesized via conventional solid state route technique. Room temperature X-ray diffraction (XRD) is performed using Bruker D2 PHASER Desktop Diffractometer (Cu-K$\alpha$, = 1.54 $\AA$) and the phase purity of prepared samples was confirmed by comparing the Rietveld refined XRD pattern with calculated model pattern using FULLPROF software package [1]. To verify the valence states of chromium and samarium ions, X-ray photoemission spectroscopy (XPS) measurements were carried out using Al-K$\alpha$ (E = 1486.7eV) lab-source. Details of sample preparation, phase confirmation and valence state determination are discussed in ref[2]. Magnetometric measurements are performed using commercial SQUID-VSM (MPMS-7T) magnetometer manufactured by Quantum Design, USA. Temperature dependent magnetization is measured in conventional zero field cooled (ZFC), field cooled cooling (FCC) and field cooled warming (FCW) modes as well as in non-conventional protocols defined in results section. The trapped remnant magnetic field inside superconducting magnet can mimic magnetization reversal [3, 4, 5] thus it is very crucial to reduce the absolute value of trapped field as low as possible. One possible way to reduce the remnant magnetization using *de-Gauss* method, in which the maximum possible magnetic field is set to zero in oscillatory mode with maximum possible field ramp rate. Following de-Gauss method, the trapped field can be reduced to $\sim$ 2Oe. Another alternative is to use 'reset magnet′ option provided by MPMS to warm the winding of electromagnet above superconducting temperature. This method can effectively reduce the value of trapped field below 0.1 Oe. Before measuring, initially we mounted standard diamagnetic sample Indium and magnet is switched to reset mode. The magnetic moment of indium is measured in presence of 2 Oe applied field at 10K. From the sign of magnetic moment of indium, it is ensured that the trapped magnetic field is positive. Afterwards, the sample is inserted inside magnetometer at room temperature and slowly cooled till 5 K with 10-15 K/minute rate. This experimental condition is mentioned as 'zero field′ everywhere in the present report. A measuring field is then applied and magnetization is recorded in warming cycle. For all other measurements protocols used here, we have *de-Gaussed* the trapped magnetic field and ensured the sign of trapped magnetic moment using standard Indium sample followed by insertion of sample in magnetometer at room temperature. Neutron diffraction data at variable temperatures ranging from 2 K- 300 K, were recorded from two axis diffractometer at D4 (Disordered materials diffractometer)[6] in ILL, Grenoble using the wavelength of 0.4994$\AA$ obtained by reflection of a Cu(220) monochromator. The low energy neutron cross-section of natural Sm is dominated by very strong resonance at 0.098 eV of $^{149}$Sm isotope[7]. To overcome the high absorption, we tuned the incident neutron energy to much higher value ($\approx$0.3eV) than the resonance energy. Further important details regarding neutron diffraction measurements are discussed in ref[8].

# 2 Evolution of magnetic phases

$SmCrO_3$ crystallizes in distorted othrohmbic structure *Pbnm* space group. The lattice parameters are described as $\sqrt{a_p}$, $\sqrt{a_p}$, 2a$_c$, where a$_p$ = 3.86(2) $\AA$ and 3.83(1) $\AA$ is the average pseudo-cubic lattice parameter at room temperature estimated by NPD and XRD, respectively[8, 2]. Fig.1(a) shows the temperature driven magnetization curves of $SmCrO_3$ measured in ZFC, FCC and FCW modes, in presence of $\mu_0$H = 0.05 T applied field. The first magnetic transition at $T_N$ = 191 K is attributed to ordering of chromium sub-lattices into canted antiferromagnetic structure. The sharp drop in magnetic moment at 34 K is assigned as spin reorientation phase transition (SRPT). As described in our previous neutron diffraction study[8], the chromium ions order in $\Gamma_4$ $\equiv$$G_x$, $A_y$, $F_z$ configuration below $T_N$, where the uncompensated moment lie along z‖c axis, whereas $\Gamma_1$ $\equiv$ $A_x$, $G_y$, $C_z$ is the observed magnetic structure below 10 K. In the vicinity of SRPT the co-existence of both $\Gamma_1$ and $\Gamma_4$ phases is observed. Across SRPT, the competition of magneto crystalline anisotropy with antisymmetric and anisotropic $Sm^{3+}$- $Cr^{3+}$ exchange interactions lead to discontinuous flipping of moment in ab-bc plane. The signatures of magnetic glassy state are observed below 15 K in bulk magnetometry results[2].

# 3 Effect of various cooling fields on M(T)

The present magnetic state of any system can be described as a function of microscopic spin configuration in ground state along with a number of independent externally imposed thermodynamic perturbations including variations in temperature, pressure, magnetic or electric field etc. Besides the instantaneous variables, the magnetically ordered materials tend to possess a functional dependency on the previous magnetic state $\mathbf{M_{t=t_0}}$, called as remnant magnetization, which is the vector resultant of the trapped magnetic moment of previous state. The *memorized* remnant magnetization is caused by the domains trapped in metastable state and not having sufficient energy to overcome the potential barrier $\nu K_U M_s/2$, where $\nu$, $M_s$ and $K_U$ are the dimension of domain, spontaneous magnetization and magneto-crystalline anisotropy, respectively. Depending on the grain size distribution, for a particular grain, the energy barrier can be compatible to thermal energy fluctuations $k_B$T, and, hence the remnant magnetization can decay by infinitesimal thermal agitation as

$$M_r = M_0 \exp[-t/\tau_0] \tag{1}$$

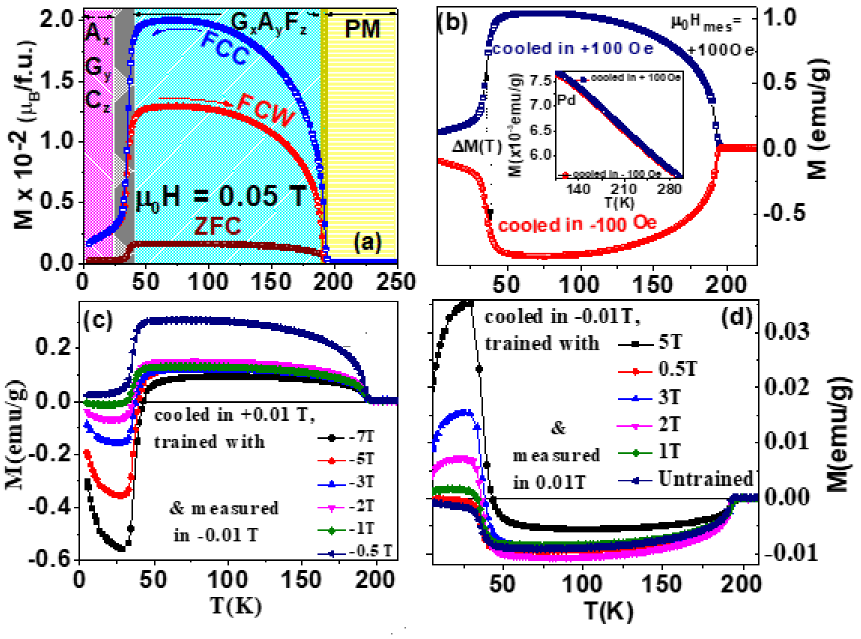

Figure 1: S(a) M(T) curves measured in ZFC, FCC and FCW cycles in presence of $\mu_0 H = 0.05T$ applied field along with temperature driven magnetic phase diagram revealing the thermal evolution of magnetic configurations. S(b) Temperature dependent response of magnetic moment when cooled in presence of $\mu_0 H_{CF}$ magnetic field and measured in presence of magnetic field equal but opposite in direction $\mu_0 H_{MF} = -\mu_0 H_{CF}$. S(c) and S(d) Training field effect: see text for detail about measuring protocols.

where $\tau_0$ is the characteristic relaxation time of single grain. Bulk magnetization comprises both instantaneous $\mathbf{M_t}$ and remnant magnetization $\mathbf{M_{t=t_0}}$ and at any particular time the ratio of instantaneous and remnant magnetization depends on the value of $\tau_0$ and external magnetic field. Only in case of relaxation time $\tau_0$ significantly longer than experimental time scale, we can observe the imprints of magnetic history $\mathbf{M_{t=t_0}}$ in the instantaneous magnetization $\mathbf{M_t}$. Here, we intend to monitor the effective contributions of instantaneous and previous magnetization in total bulk magnetization, with respect to different cooling (previous) and measuring (instantaneous) field values. With this motive, two sets of experiments are performed, as shown in Fig.1(b) . In first experiment, we cooled the sample from room temperature to 5 K in presence of cooling field $\mu_0 H_{CF}$ = - 0.01 T. At 5 K the field is switched to measuring field value $\mu_0 H_{MF}$ = + 0.01 T, and magnetic moment is recorded in warming mode from 5 K-300 K. Secondly, we reversed the $\mu_0 H_{CF}$ to be + 0.01 T and again measured the data in warming mode with same field $\mu_0 H_{MF}$ = + 0.01 T . Clearly, the sign of magnetic moment is not bounded to the instantaneous measuring field, but governed by the field in which it was cooled previously. The same set of experiments are performed with standard para-magnetic cylindrical palladium sample to estimate the maximum possible instrumental error caused by any trace of trapped field in superconducting solenoid and noise signals caused by sample holder and sample environment. The negligible difference between two curves; ΔM is $\sim 10^{-5}$ emu/g, which is four order less in magnitude with comparison to the maximum value of ΔM $\sim$ 0.4 emu/g in $SmCrO_3$, points toward the reliability of these measurements. In the next series of experiments, we demonstrate the stability of *memorized* magnetization by training the system with application of high magnetic field. The protocol followed for these measurements are as follows: we firstly cooled the sample in $\mu_0 H_{CF}$= +0.01 T down to 5 K and then switched a negative training field with value much higher than absolute value of $\mu_0 H_{CF}$. We held this training field for 500 seconds, allowing the magnetic domains to come in equilibrium state. Then we switched off the training field and measured the magnetization while warming with positive value of $H_{CF}$. As shown in Fig.1(c), although the training field flips the net magnetic moment in positive direction below $T_{SRPT}$, but it is still not able to erase the stored cooling field effect and the magnitude of moment again becomes negative for temperatures just above $T_{SRPT}$. The similar situation is observed in the vice-versa situation, reversing the sign of cooling field, training field and measuring fields as shown in Fig.1(d).For a single domain grain, the mean magnetic moment at any temperature $T_0$ can be written as:

$$M(T_0) = \nu M_s(T_0) tanh(M_s(T) H_{MF}(T)/kT) \tag{2}$$

which depends on value of applied field $H_{MF}$ acting at temperature T when critical diameter becomes equal to the dimensions of grain[9]. The complexity with the above described phenomenological understanding of TRM starts arising when we look towards microscopic insight of underlying mechanism. Based on the magnetometric experiments, we have tried to formulate the empirical functional dependency of magnetization in $SmCrO_3$. The magnetization can be written as convolution of two parts : memory independent $M_{FCW}$(T, $H_{MF}$) and memory dependent remnant part

which is the function of previous state parameters, as follows:

$$M(T) = M_{FCW}(T, H_{MF}) \bullet [c_0 + ce^{-\alpha T}] \tag{3}$$

Where the coefficients $c_0$, c and $\alpha$ are defined as;

$$c_0 = 1/(1-\gamma); H_{MF} \neq H_{CF}$$
$$c_0 \approx 0.85(3); H_{MF} = H_{mem}$$
$$\alpha \equiv A_0 + A_1\gamma + A_2\gamma^2 + A_3\gamma^3$$
$$\gamma = |H_{MF}|/H_{mem}|$$

and $M_{FCW}$ is the FCW M(T) at applied field value $\mu_0 H$ = $M_{MF}$, $\mu_0 H_{CF}$ is the cooling field while sweeping temperature window $\Delta W_T$. The exponential coefficient c is a thermodynamic constant for the system and its value is $\approx$ 8.35*$10^{-5}$ emu/g. The value of $c_0$ or as a consequence the value of $\gamma$ modulates the sign of observed magnetic moment. The exponential factor governs the effective memory response parameter $H_{CF}$ in the thermal variation of magnetic moment.

# 4 Characteristics of magnetization relaxation

| T(K) | $\beta$ | TRM (0) | | TRM (-100 Oe) | | IRM (0) | | IRM (-100 Oe) | |
|---|---|---|---|---|---|---|---|---|---|
| | | $\sigma_{r,t_0}$ | $\tau_0$ | $\sigma_{r,t_0}$ | $\tau_0$ | $\sigma_{r,t_0}$ | $\tau_0$ | $\sigma_{r,t_0}$ | $\tau_0$ |
| 185 | 0.53479(9) | 0.01327(5) | 23.9(2) | 0.0161(2) | 13.5(2) | 0.0179(2) | 3.4(8) | 0.0299(2) | 4.4(5) |
| 180 | 0.394(7) | 0.0186(3) | 384(41) | 0.0094(7) | 555(36) | 0.0109(6) | 125(38) | 0.0102(2) | 107(11) |
| 150 | 0.33469(3) | 0.00315(3) | 1223(109) | 0.004181(9) | 3154(802) | 0.00377(7) | 719(135) | 0.00499(5) | 905(236) |

Table 1: Fitting parameters describing the magnetization relaxation with respect of time

# References


[1] J. Rodrguez-Carvajal, Recent advances in magnetic structure determination by neutron powder diffraction, *Physica B: Condensed Matter* **192** 55-69, (1993).

[2] M. Tripathi, R. J. Choudhary and D. M. Phase, , Phase coexistence and the magnetic glass-like phase associated with the Morin type spin reorientation phase transition in $SmCrO_3$, *RSC Advances* **6**, 93, 90255-90262,(2016).

[3] N. Kumar and A. Sundaresan, On the observation of negative magnetization under zero-field-cooled process. , *Solid State Communications* **150(25-26)** , 1162-1164 (2010).

[4] L. D. Tung, Tunable temperature-induced magnetization jump in a Gd V O 3 single crystal, *Physical Review B*, **73(2)**, 024428 (2006).

[5] M. Tripathi, T. Chatterji, H. E. Fisher, R. Raghunathan, S. Majumder, R. J. Choudhary and D. M. Phase, Role of local short scale correlations in the origin of negative magnetization, *Physical Review B*, **99**, 1, 014422 (2019).

[6] H. E. Fischer, G. J. Cuello, P. Palleau, D. Feltin , A. C. Barnes, Y. S. Badyal and J. M. Simonson, D4c: A very high precision diffractometer for disordered materials, *Applied Physics A*, **74**,1, s160-s162 (2002).

[7] J. E. Lynn and P. A. Seeger, Resonance effects in neutron scattering lengths of rare-earth nuclides, *Atomic Data and Nuclear Data Tables*, **44**, 2, 191-207 (1990).

[8] M. Tripathi, R. J. Choudhary, D. M. Phase, T. Chatterji, and H. E. Fischer, Evolution of magnetic phases in $SmCrO_3$: A neutron diffraction and magnetometric study, *Physical Review B*, **96**, 17, 174421 (2017).

[9] L. Néel, Some theoretical aspects of rock-magnetism, *Advances in physics*, **4**, 14, 191-243 (1955).
